# Supplementary material for: Geometric Criticality in Scale-Invariant Networks
Source: arXiv:2507.11348 source file (2026-02-04)
Supplement: Supplementary file 1 [file Supplemental_Material.pdf]

# Geometric Criticality in Scale-Invariant Networks

Lorenzo Lucarini,<sup>1,2</sup> Giulio Cimini,<sup>1,2</sup> and Pablo Villegas<sup>1,3,\*</sup>

<sup>1</sup>*Enrico Fermi Research Center (CREF), Via Panisperna 89A, 00184, Rome, Italy*

<sup>2</sup>*Dipartimento di Fisica, Università di Roma “Tor Vergata”, 00133 Rome, Italy*

<sup>3</sup>*Instituto Carlos I de Física Teórica y Computacional, Universidad de Granada, Granada, Spain*

## CONTENTS

|                                                                            |   |
|----------------------------------------------------------------------------|---|
| Summary table for geometric criticality in different networks and lattices | 2 |
| 2D lattices                                                                | 2 |
| Triangular lattice                                                         | 2 |
| Hexagonal lattice                                                          | 4 |
| 3D lattices                                                                | 6 |
| DGM networks                                                               | 7 |
| Tree networks                                                              | 8 |
| Hierarchic-Modular networks                                                | 9 |

---

\* [pablo.villegas@cref.it](mailto:pablo.villegas@cref.it)

## SUMMARY TABLE FOR GEOMETRIC CRITICALITY IN DIFFERENT NETWORKS AND LATTICES

Table I summarizes the results for the emergence of geometric criticality across various lattices and networks, considering both rewiring (preserving the total number of links) and dilution. The reported values have been estimated through a combined analysis of the heat capacity of each architecture and the correlation dimension, when the latter is interpretable (as discussed in the main text).

|          | 2D squared | 2D triangular | 2D hexagonal | 3D cubic | Trees              | DGM     |
|----------|------------|---------------|--------------|----------|--------------------|---------|
| Rewiring | 0.10(1)    | 0.17(4)       | 0.055(10)    | 0.20(5)  | $\mathcal{O}(1/N)$ | 0.05(3) |
| Dilution | 0.20(5)    | 0.25(1)       | 0.11(2)      | 0.55(5)  | 1                  | 0.15(5) |

Table I. Perturbation thresholds for different lattices and networks. Parentheses indicate the estimated uncertainty.

### 2D LATTICES

#### Triangular lattice

We present a detailed analysis for the case of 2D triangular lattices here. Fig. 1 reports finite-size scaling analyses confirming the existence of a finite critical rewiring probability in the thermodynamic limit,  $p_{r,c} = 0.17(4)$ . This defines, as in the case of the square lattice, the attraction basin of the 2D triangular lattice under the introduction of shortcuts. Note that, the expected value of  $p_{r,c}$  is dependent of the specific lattice tiling.

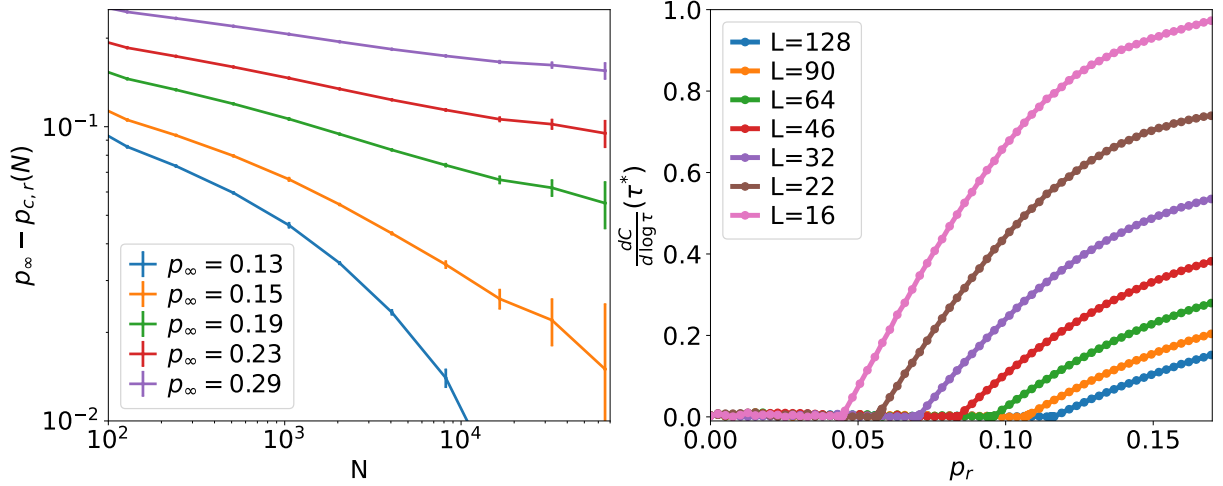

Figure 1. Shortcuts in 2D triangular lattices. **(Left)** Finite-size scaling analysis of the vanishing heat capacity peaks. The distance of the size-dependent peak locations  $p_{r,c}(N)$  from their asymptotic value for  $N \rightarrow \infty$ ,  $p_{r,c}^\infty$ , scales as a power law of the system size, only at  $p_{r,c}^\infty = 0.17(4)$ , revealing the existence of true scaling at criticality. **(Right)** First derivative of the heat capacity at the first peak versus rewiring probability,  $p_r$ , for different lattice sizes (see legend).

For 2D triangular lattices, the analysis of heat capacity versus dilution probability enables the identification of the specific transition point,  $p_{d,c}$ , at which the ultraviolet cut-off  $\Lambda$  vanishes. We detect this geometric breakdown by analyzing the curvature (concavity) of the first peak in the heat capacity (see Fig. 2(a)), as illustrated in Fig. 2(b). The correlation dimension of this lattice as a function of the rewiring probability is reported in Fig. 2(c). In particular, the dimension extracted from the scaling  $C(\ell) \propto \ell^D$  is shown in Fig. 2(d). Note that beyond  $p_{d,c}$ , the effective dimension of the network decreases progressively toward the RT value  $d_s = 4/3$  at  $p_c$ .

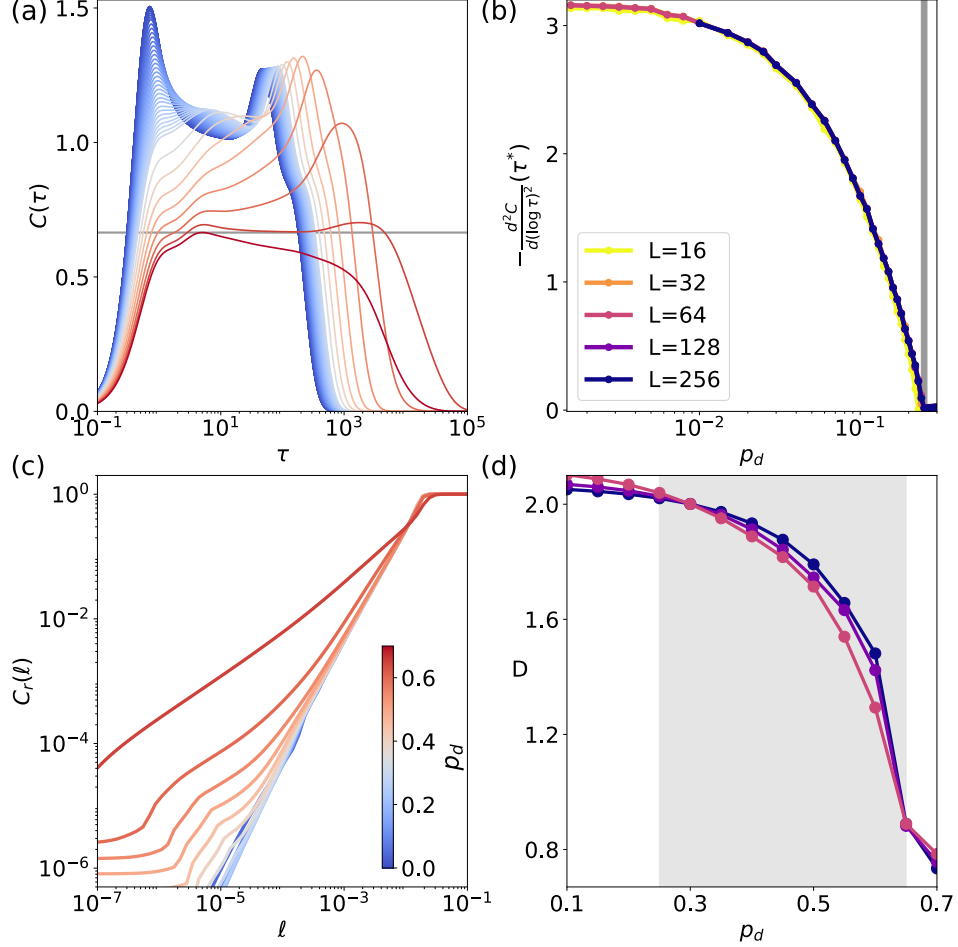

Figure 2. Diluted 2D triangular lattices. **(a)** Heat capacity,  $C$ , versus diffusion time,  $\tau$ , for different dilute probabilities (see colorbar). The gray line represents the expected plateau for a RT. **(b)** Second derivative of the heat capacity at the first peak versus dilute probability,  $p_d$ , for different lattice sizes (see legend). The vertical gray line represents the point where the 2D ultraviolet cut-off is expected to disappear. **(c)** Correlation integral  $C_r(\ell)$  as a function of the distance  $\ell$  for different dilute probabilities (see colorbar). **(d)** Estimated correlation dimension,  $D$ , versus dilution probability,  $p_d$  for different lattice sizes. The gray area represents dilute probabilities between  $p_{d,c}$  and the percolation threshold. All curves have been averaged over  $10^3 - 10^4$  realizations.

### Hexagonal lattice

For the case of 2D hexagonal lattices, Fig. 3 reports finite-size scaling analyses confirming the existence of a finite critical rewiring probability in the thermodynamic limit,  $p_{r,c} = 0.055(10)$ . This defines, as in the case of the square lattice, the attraction basin of the 2D hexagonal lattice under the introduction of shortcuts. Note that the expected value of  $p_{r,c}$  depends on the specific lattice tiling.

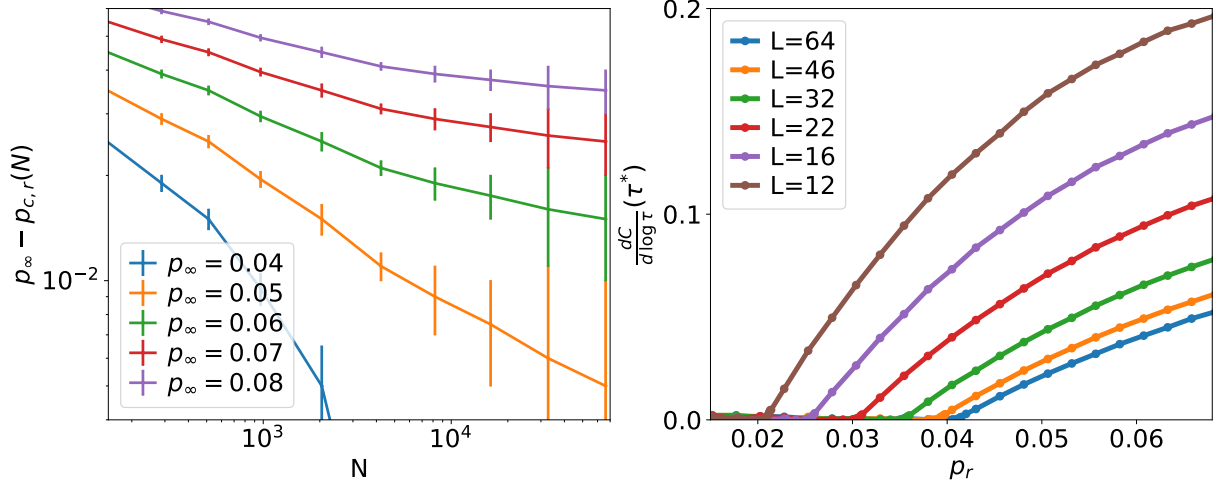

Figure 3. Shortcuts in 2D hexagonal lattices. **(left)** Finite-size scaling analysis of the vanishing heat capacity peaks. The distance of the size-dependent peak locations  $p_{r,c}(N)$  from their asymptotic value for  $N \rightarrow \infty$ ,  $p_{r,c}^\infty$ , scales as a power law of the system size, only at  $p_{r,c}^\infty = 0.055(10)$ , revealing the existence of true scaling at criticality. **(right)** First derivative of the heat capacity at the first peak versus rewiring probability,  $p_r$ , for different lattice sizes (see legend).

For 2D hexagonal lattices, the analysis of heat capacity as a function of dilution probability allows us to identify the specific transition point,  $p_{d,c}$ , where the ultraviolet cut-off  $\Lambda$  vanishes. This geometric breakdown is identified by examining the curvature (concavity) of the first peak in the heat capacity (see Fig. 2(a)), as illustrated in Fig. 2(b). The correlation dimension of the lattice as a function of the rewiring probability is shown in Fig. 2(c), while the dimension extracted from the scaling  $C(\ell) \propto \ell^D$  is reported in Fig. 2(d). Notably, beyond  $p_{d,c}$ , the effective dimension of the network gradually decreases toward the RT value  $d_s = 4/3$  at  $p_c$ .

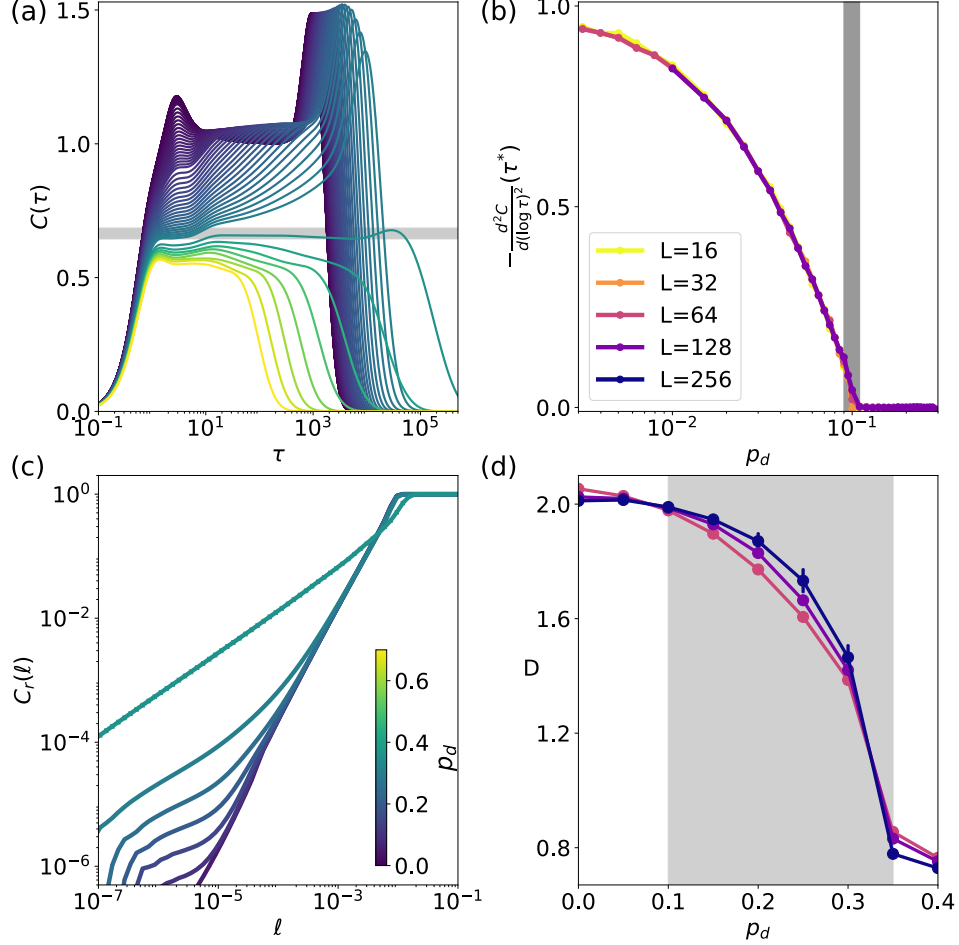

Figure 4. Diluted 2D hexagonal lattices. **(a)** Heat capacity,  $C$ , versus diffusion time,  $\tau$ , for different dilute probabilities (see colorbar). The gray line represents the expected plateau for a RT. **(b)** Second derivative of the heat capacity at the first peak versus dilute probability,  $p_d$ , for different lattice sizes (see legend). The vertical gray line represents the point where the 2D ultraviolet cut-off is expected to disappear. **(c)** Correlation integral  $C_r(\ell)$  as a function of the distance  $\ell$  for different dilute probabilities (see colorbar). **(d)** Estimated correlation dimension,  $D$ , versus dilution probability,  $p_d$  for different lattice sizes. The gray area represents dilute probabilities between  $p_{d,c}$  and the percolation threshold. All curves have been averaged over  $10^3 - 10^4$  realizations.

## 3D LATTICES

The inclusion of shortcuts in a 3D cubic lattice is analyzed in Fig. 5. Here, we report again the finite-size scaling analyses confirming the existence of a finite critical rewiring probability in the thermodynamic limit,  $p_{r,c} = 0.20(5)$ . This defines, as in the case of the 2D lattices, the attraction basin of the 3D cubic lattice under the introduction of shortcuts. Note that the expected value of  $p_{r,c}$  depends on the specific lattice tiling.

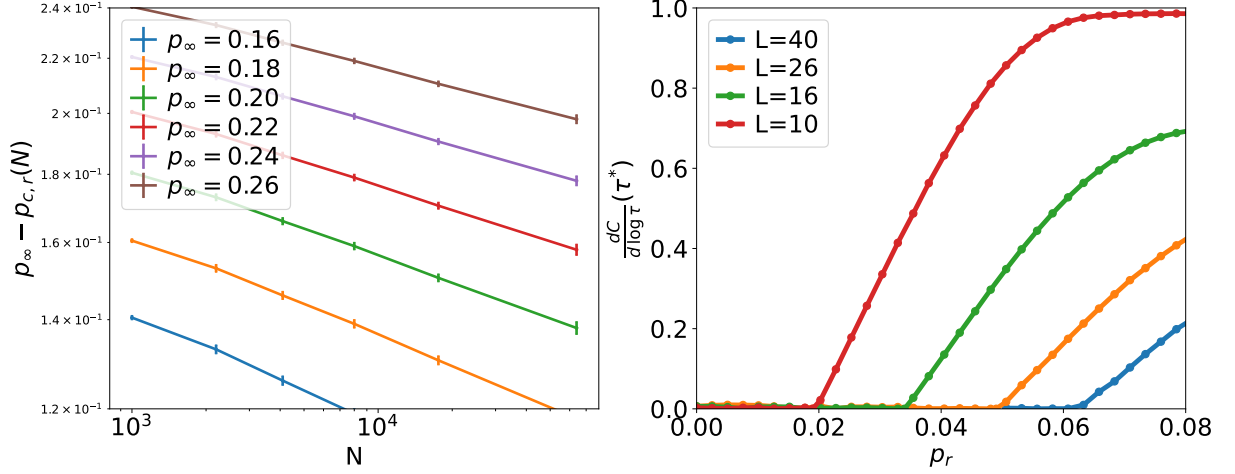

Figure 5. Shortcuts in 3D square lattices. **(Left)** Finite-size scaling analysis of the vanishing heat capacity peaks. The distance of the size-dependent peak locations  $p_{r,c}(N)$  from their asymptotic value for  $N \rightarrow \infty$ ,  $p_{r,c}^\infty$ , scales as a power law of the system size, only at  $p_{r,c}^\infty = 0.20(5)$ , revealing the existence of true scaling at criticality. **(Right)** First derivative of the heat capacity at the first peak versus rewiring probability,  $p_r$ , for different lattice sizes (see legend).

For 3D cubic lattices, the analysis of heat capacity as a function of dilution probability allows us to identify the specific transition point,  $p_{d,c}$ , where the ultraviolet cut-off  $\Lambda$  vanishes. This geometric breakdown is identified by examining the curvature (concavity) of the first peak in the heat capacity (see the left part of Fig. 6). The correlation dimension of the lattice as a function of the rewiring probability is shown in Fig. 6, while the dimension extracted from the scaling  $C(\ell) \propto \ell^D$  is reported in the rightmost part of Fig. 6. Notably, beyond  $p_{d,c}$ , the effective dimension of the network gradually decreases toward the RT value  $d_s = 4/3$  at  $p_c$ .

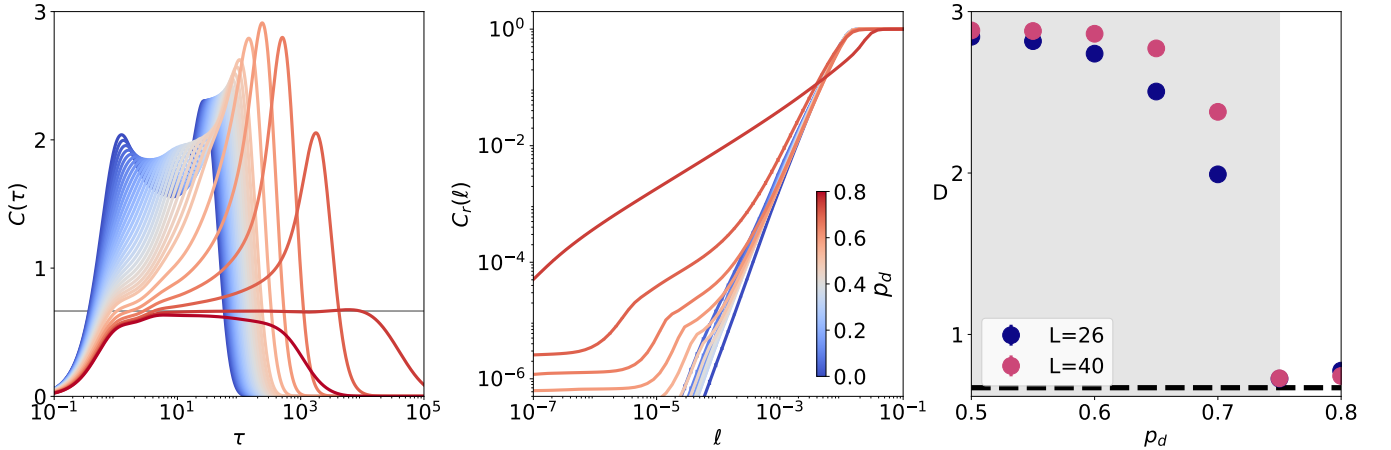

Figure 6. Diluted 3D square lattices **(Left)** Heat capacity,  $C$ , versus diffusion time,  $\tau$ , for different dilute probabilities (see colorbar). The gray line represents the expected plateau for a RT. **(Center)** Correlation integral  $C_r(\ell)$  as a function of the distance  $\ell$  for different dilute probabilities (see colorbar). **(Right)** Estimated correlation dimension,  $D$ , versus dilution probability,  $p_d$  for different lattice sizes. Inset: Correlation integral  $C(\ell)$  vs distance  $\ell$  for different dilute probabilities. The gray area represents dilute probabilities between  $p_{d,c}$  and the percolation threshold. All curves have been averaged over  $10^3 - 10^4$  realizations.

## DGM NETWORKS

We now move on to the case of rewiring or shortcuts in DGM networks, as shown in Fig. 7. Finite-size scaling analyses confirm the existence of a finite critical rewiring probability in the thermodynamic limit,  $p_{r,c} = 0.05(3)$ . It is possible to observe that  $p_\infty = 0.03$  exhibits a convergence to zero when the system size increases. We emphasize that considering  $p_\infty = 0.02$  generates an exponential decay as a function of the system size. This defines the example of an attraction basin for a scale-invariant network under the introduction of shortcuts.

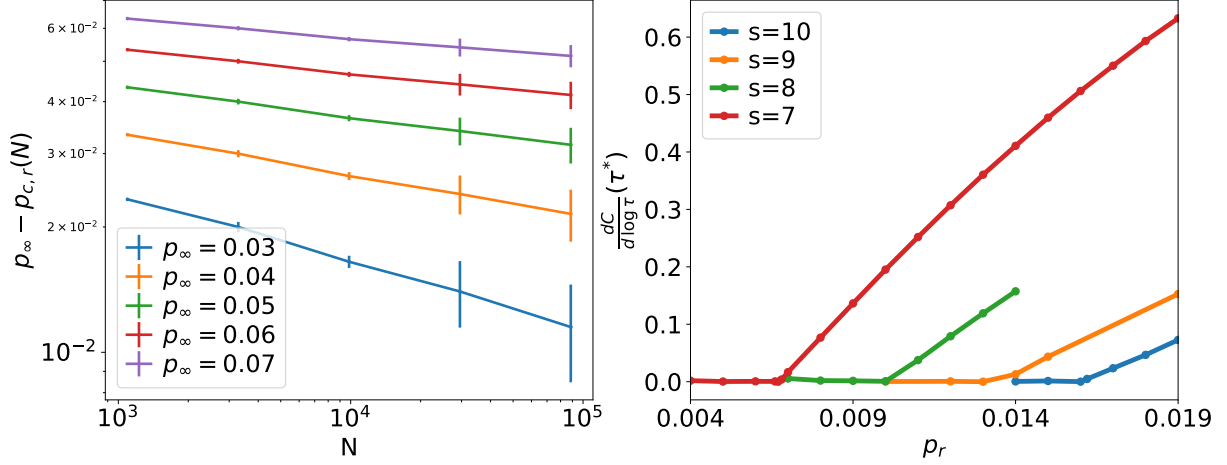

Figure 7. Shortcuts in DGM networks. **(left)** Finite-size scaling analysis of the vanishing heat capacity peaks. The distance of the size-dependent peak locations  $p_{r,c}(N)$  from their asymptotic value for  $N \rightarrow \infty$ ,  $p_{r,c}^\infty$ , scales as a power law of the system size, only at  $p_{r,c}^\infty = 0.05(3)$ , revealing the existence of true scaling at criticality. **(right)** First derivative of the heat capacity at the first peak versus rewiring probability,  $p_r$ , for different levels  $s$  (see legend).

Fig. 8 shows the correlation integral for different values of the dilution probability in a DGM network of size  $N = 29526$ . For low dilution probabilities, the network exhibits a spectral dimension consistent with the expected theoretical value, which progressively deviates and eventually collapses for high dilution.

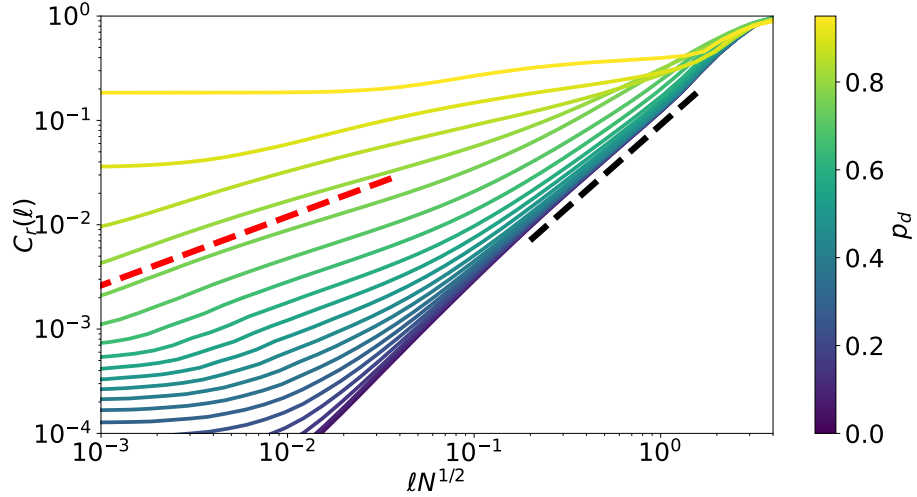

Figure 8. Correlation integral  $C_r(\ell)$  as a function of the rescaled distance  $\ell\sqrt{N}$  for DGM networks with structural level  $s = 10$ , subjected to dilution with different dilution probabilities (see legend). Dashed lines are guides to the eye indicating the slopes corresponding to correlation dimensions  $D = 2/3$  and  $D = \frac{3.17}{2}$ .

Figure 9 presents the percolation properties of a diluted DGM network. The leftmost figure shows the average fraction of nodes belonging to the giant component as a function of the dilution probability for different hierarchical levels  $s$  (see legend). As the dilution increases, the giant component progressively disappears, with a critical percolation threshold approaching one (see below). Still, the standard deviation of the percolation order parameter highlights the fluctuations associated with the percolation transition. The peak indicates the true critical point where these networks exhibit a percolation transition,  $p = 0.95(5)$ . Finite-size scaling analysis of the percolation threshold across different values of  $s$  permits us to confirm that the critical point is slightly lower than one.

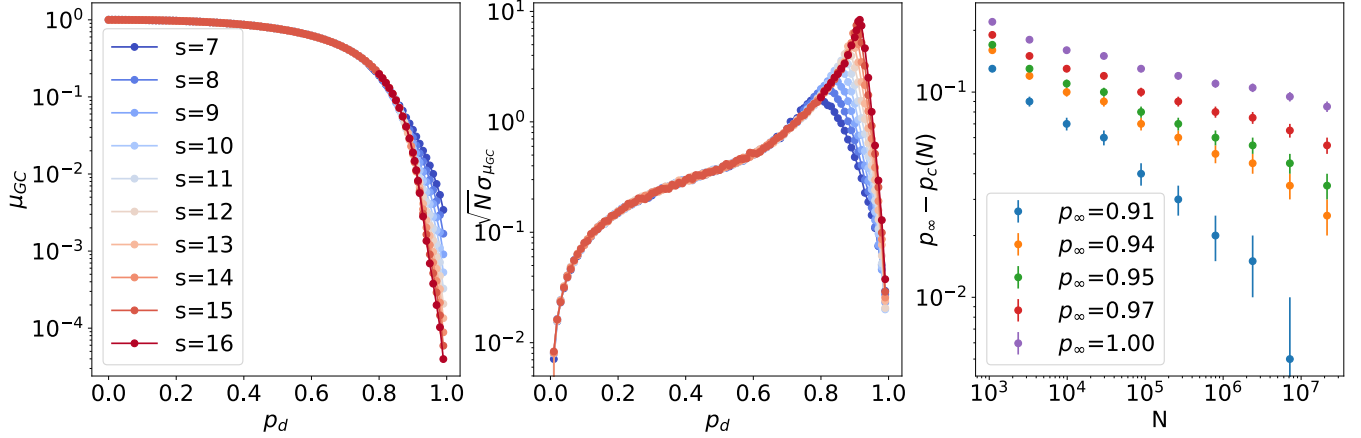

Figure 9. DGM Percolation Threshold. **(left)** Average fraction of number of nodes in the giant component for a diluted DGM network as a function of the dilution probability. Different curves correspond to different values of level  $s$  (see legend). **(center)** Standard deviation of the fraction of number of nodes in the giant component for a diluted DGM network as a function of the dilution probability. Different curves correspond to different values of level  $s$  (see legend). **(right)** Finite-size scaling analysis of the percolation threshold.

### TREE NETWORKS

Here, we report the percolation transition as a function of the rewiring probability for random trees and Barabási–Albert networks. Both cases are topologically similar to 1D rings, as they also lack loops. Notably, in all three cases, the critical probability required to present a giant connected component vanishes in the thermodynamic limit. This is revealed by the collapse of the curves when properly rescaled with  $N$ , as shown in Fig. 10.

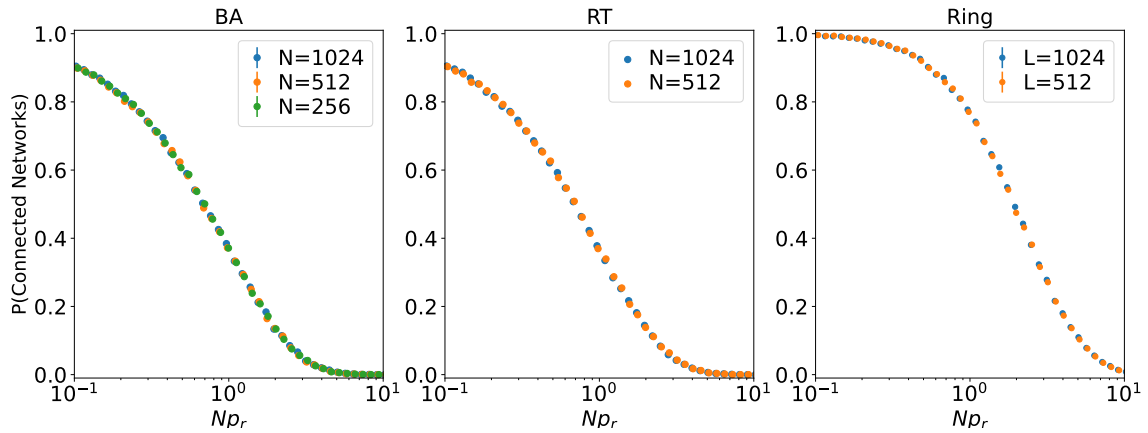

Figure 10. Percentage of connected networks as a function of  $p_r N$ , where  $p_r$  is the rewiring probability and  $N$  the number of nodes. From left to right: Barabási–Albert networks with  $m = 1$ , random trees, and ring graphs. Different curves correspond to different values of  $N$  (see legend).

# HIERARCHIC-MODULAR NETWORKS

Figure 11 illustrates the percolation behavior of diluted HMNs across different hierarchical levels  $s$ . The leftmost panel shows the average fraction of nodes in the giant component as a function of the dilution probability. As dilution increases, the network undergoes a complex percolation transition. In particular, the analysis of the standard deviation of the percolation order parameter (center panel) reveals that these networks exhibit a broad critical region, with fluctuations diverging in the thermodynamic limit even at low values of  $p_d$ . This suggests the presence of persistent critical fluctuations that constrain the lacunarity of the network across the entire range of  $p$ . Finally, the rightmost panel shows the heat capacity  $C$  as a function of diffusion time  $\tau$  for various dilution probabilities (see colorbar).

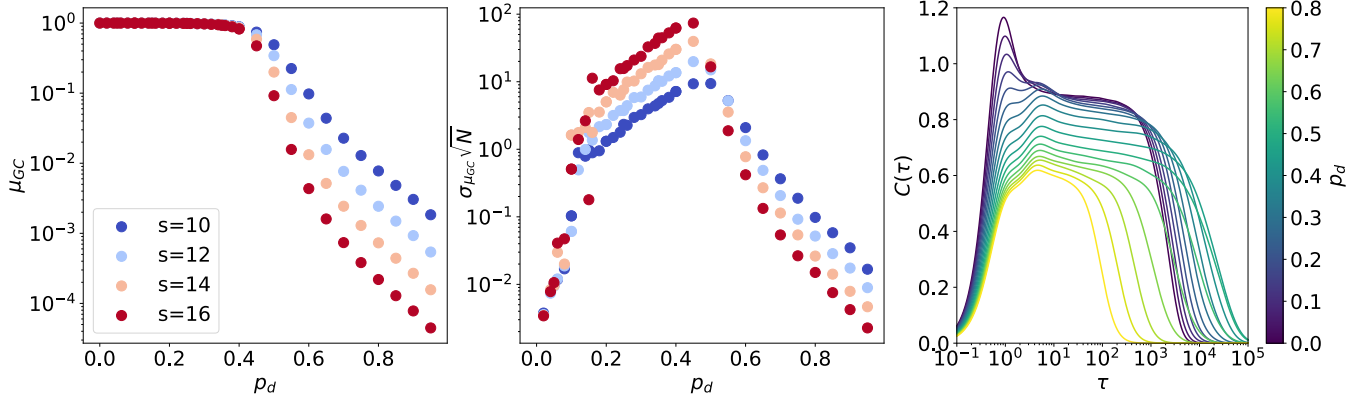

Figure 11. HMN Percolation Threshold. **(Left)** Average fraction of the number of nodes in the giant component for a diluted HMN as a function of the dilution probability. Different curves correspond to different values of level  $s$  (see legend). **(Center)** Standard deviation of the fraction of the number of nodes in the giant component for a diluted HMN as a function of the dilution probability. Different curves correspond to different values of level  $s$  (see legend). **(Right)** Heat capacity,  $C$ , versus diffusion time,  $\tau$ , for different dilute probabilities (see colorbar).
